# Supplementary material for: Fair Contrastive Learning for Facial Attribute Classification
Source: arXiv:2203.16209 source file (2022-03-30)
Supplement: Supplementary file 2 [file table_gan_appendix.tex]

\begin{table}[t]
\centering
\resizebox{0.47\textwidth}{!}{
\begin{tabular}{cccc} \toprule
Method & Ramaswamy \textit{et al.}~\cite{FairGen} & EO ($\downarrow$) & Acc. ($\uparrow$) \\ \cmidrule[0.5pt]{1-4} \morecmidrules\cmidrule[0.5pt]{1-4}
\multirow{2}{*}{\textit{Cross-Entropy}~\cite{resnet}} & \xmark & 5.8$_{\pm 0.8}$ & 91.6$_{\pm 0.3}$ \\ \cmidrule[0.3pt]{2-4}
 & \cmark & 4.5$_{\pm 0.7}$ & 91.4$_{\pm 0.4}$ \\ \cmidrule[0.3pt]{1-4}
\multirow{2}{*}{\textit{FSCL+}} &  \xmark & 3.1$_{\pm 0.1}$ & 91.6$_{\pm 0.1}$ \\ \cmidrule[0.3pt]{2-4}
 & \cmark & \textbf{2.5}$_{\pm 0.1}$ & 91.9$_{\pm 0.1}$ \\ \bottomrule
\end{tabular}
}
\caption{\textbf{Compatibility with Fair Data Augmentation}~\cite{FairGen}. We set $smiling$ and $male$ to the target class and sensitive attribute, respectively, on CelebA dataset.}
\label{table:gan}
\end{table}
